# Supplementary material for: Towards Practical Meshlet Compression
Source: arXiv:2404.06359 source file (2024-08-13)
Supplement: Supplementary file 1 [file appendix.tex]

\section{Appendix}\label{Sec:App}
In case
